# Supplementary material for: Generate, Annotate, and Learn: NLP with Synthetic Text
Source: arXiv:2106.06168 source file (2022-05-31)
Supplement: Supplementary file 1 [file appendix.tex]

\clearpage\newpage
% \onecolumn

\counterwithin{figure}{section}
\counterwithin{table}{section}

% \section{Pseudo-code of Algorithms}
% \label{sec:app:alg}

% \input{alg-selftrain}
% \input{alg-gest}

\section{GAL on Image Classification Tasks}
\label{app:ic-task}

As a proof of concept, in addition to NLP and tabular tasks, we assess the effectiveness of \gal on CIFAR-10 \citep{cifar} and Fashion MNIST \citep{xiao2017fashion} as well. We adopt the
NCSN model of~\cite{song2019generative_ncsn} as the task-specific generative model.
We use the CIFAR-10 model provided by the authors and train a model on Fashion MNIST using the same configuration as CIFAR-10.
We select the model checkpoint resulting in the best FID score vs. training set~\citep{heusel2017gans} based on 1000 samples.
We then use the NCSN models to generate up to 10$\times$ synthetic unlabeled data, \ie~500K for CIFAR-10 and 600K for Fashion MNIST.
See Appendix~\ref{sec:example} for representative samples.

\input{tab-cv-cifar10}
We adopt FixMatch~\citep{sohn2020fixmatch} to conduct semi-supervised learning on vision tasks, since
FixMatch has shown promising results on CIFAR-10.
Specifically, we train a classifier on mini-batches of intertwined labeled and unlabeled data (synthetic).
In each iteration, we obtain pseudo-labels for the unlabeled data, but filter unlabeled examples based on classifier's confidence, 
\ie examples are kept on which the largest class probability exceeds $\tau$.
Weak augmentation is used to define pseudo labels, but strong augmentations are used to obtain student model's predictions.
%We minimize the loss on the selected synthetic  against the prediction of the model for strongly augmented versions of them.
We randomly sample from the strong augmentations list defined in RandAugment~\citep{cubuk2020randaugment}.
We only apply strong augmentations to the synthetic samples and not the original labeled data 
to ensure a fair comparison with the baseline. % (\ie with no synthetic data) where no strong augmentations were used. 

We conduct experiments on three different convolutional neural network architectures: VGG19~\citep{simonyan2014very_vgg}, WideResnet28-10~\citep{zagoruyko2016_wideresnet}, and ResNet110~\citep{he2016deep_resnet}.
For the full list of hyperparameters and other implementation details, please refer to Appendix~\ref{sec:training_details}.
Each classifier is trained for 200 epochs and 3 synthetic datasets of size ($1\times$, $5\times$, $10\times$) of the training dataset are used.

Table~\ref{tab:cv-cifar10} shows that \gal achieves an average error reduction of $0.78\%$ over the baseline on CIFAR-10 across the 3 architectures tested.
Further, it appears that the larger the synthetic dataset size, the better the performance of \gal is.
We note that the reported results are the average of 3 independent runs.
%Notably, we achieve almost 1\% improvement on VGG19 architecture.
Similarly on Fashion MNIST, we witness consistent gains across all architectures. 
Fashion MNIST results are included in Appendix~\ref{sec:additional}.
Our image classification experiments confirm that even when the generative model of \gal is not pretrained on open domain data and solely trained on the dataset at hand,
\gal can offer significant improvements.

\tabref{tab-cv-fashion} presents \gal results on Fashion MNIST dataset. Similar to CIFAR-10, we observe a performance improvement across the three architectures.   
\input{tab-cv-fashion}

\newpage 
\section{Generated Unlabeled Examples Annotated with Pseudo Labels}
\label{sec:example}

\begin{figure*}[h!]
 %\small
 \centering
 \begin{tabular}{@{}r@{\hspace{.2cm}}c@{}}
 \raisebox{.85cm}{truck} & \includegraphics[width=0.88\textwidth]{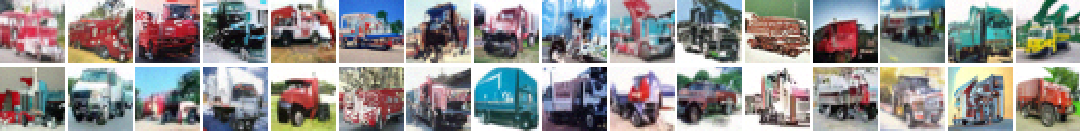} \\
 \raisebox{.85cm}{ship} & \includegraphics[width=0.88\textwidth]{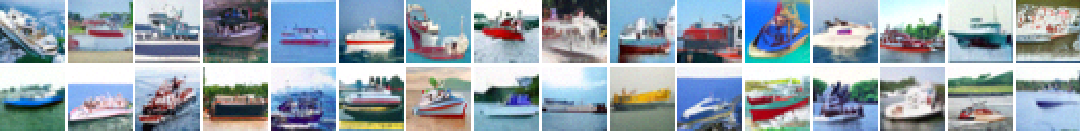} \\
 \raisebox{.85cm}{horse} & \includegraphics[width=0.88\textwidth]{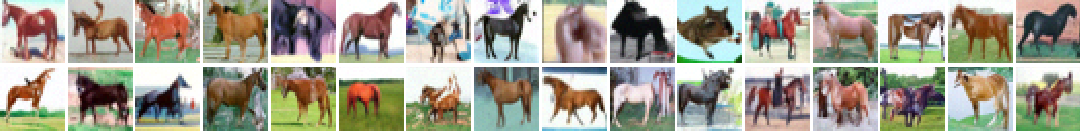} \\
 \raisebox{.85cm}{frog} & \includegraphics[width=0.88\textwidth]{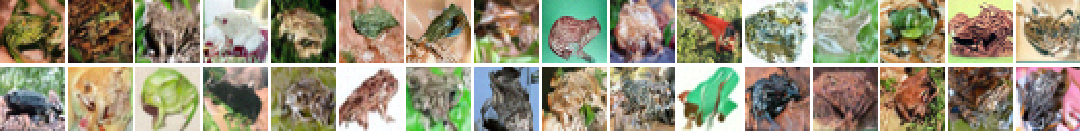} \\
 \raisebox{.85cm}{dog} & \includegraphics[width=0.88\textwidth]{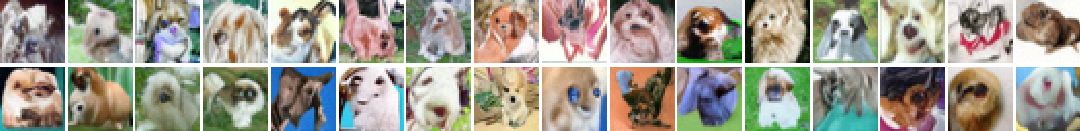} \\
 \raisebox{.85cm}{deer} & \includegraphics[width=0.88\textwidth]{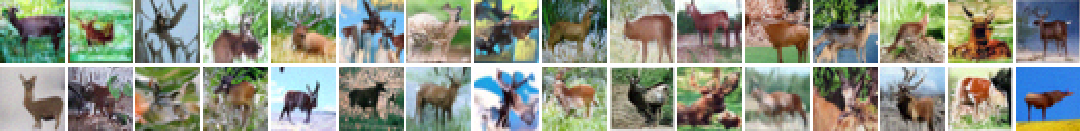} \\
 \raisebox{.85cm}{cat} & \includegraphics[width=0.88\textwidth]{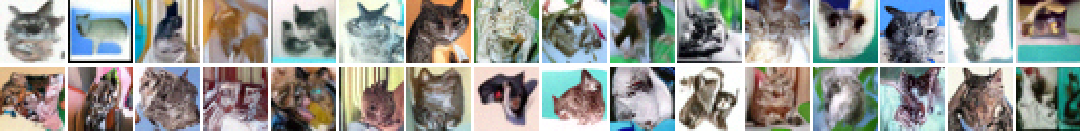} \\
 \raisebox{.85cm}{bird} & \includegraphics[width=0.88\textwidth]{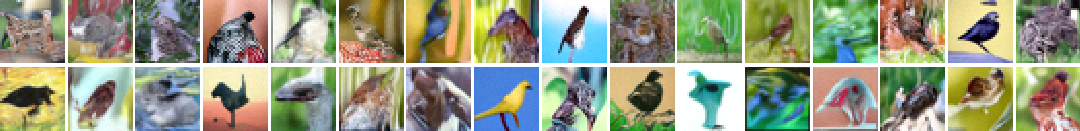} \\
 \raisebox{.85cm}{car} & \includegraphics[width=0.88\textwidth]{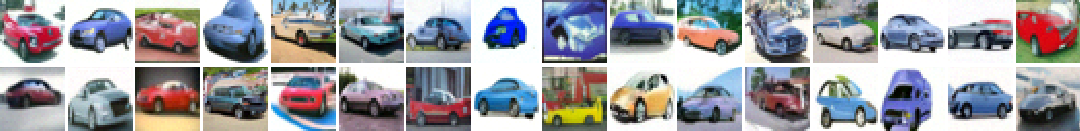} \\
 \raisebox{.85cm}{airplane} & \includegraphics[width=0.88\textwidth]{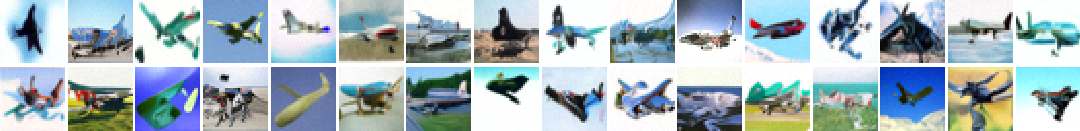}
\end{tabular}
\caption{CIFAR-10 synthetic samples generated by NCSN~\citep{song2019generative_ncsn} and corresponding pseudo-labels. Images are filtered based on a confidence threshold of $\tau = 0.95$ and categorized based on pseudo-labels. For each category, 16 random samples are shown.}
\label{fig:synth_examples_cifar10}
\end{figure*}

\begin{figure*}[h!]
 %\small
 \centering
 \begin{tabular}{@{}r@{\hspace{.2cm}}c@{}}
 \raisebox{.3cm}{boot} & \includegraphics[trim={0 2.28cm 0 0},clip,width=0.88\textwidth]{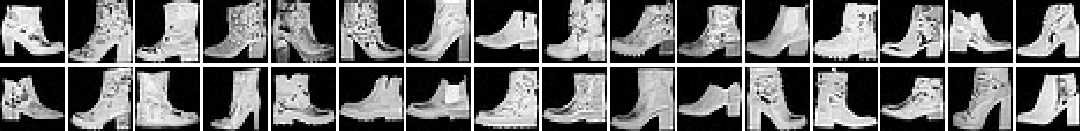} \\
 \raisebox{.3cm}{bag} & \includegraphics[trim={0 2.28cm 0 0},clip,width=0.88\textwidth]{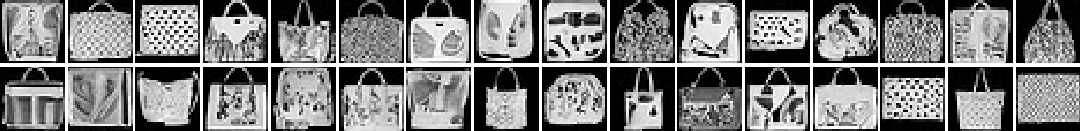} \\
 \raisebox{.3cm}{sneaker} & \includegraphics[trim={0 2.28cm 0 0},clip,width=0.88\textwidth]{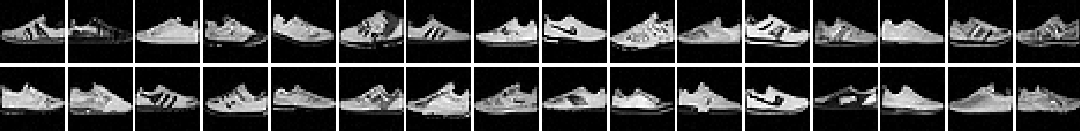} \\
 \raisebox{.3cm}{shirt} & \includegraphics[trim={0 2.28cm 0 0},clip,width=0.88\textwidth]{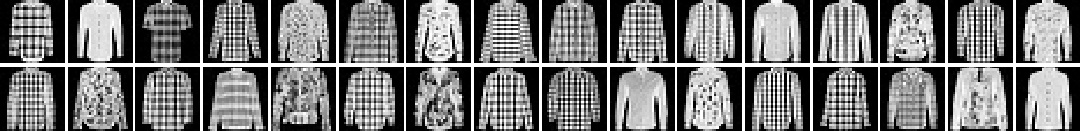} \\
 \raisebox{.3cm}{sandal} & \includegraphics[trim={0 2.28cm 0 0},clip,width=0.88\textwidth]{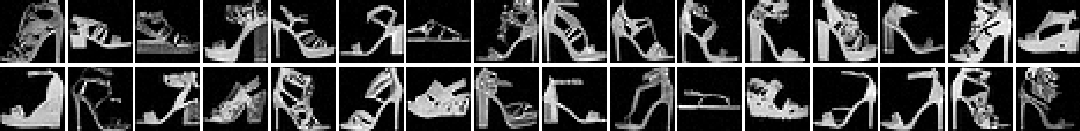} \\
 \raisebox{.3cm}{coat} & \includegraphics[trim={0 2.28cm 0 0},clip,width=0.88\textwidth]{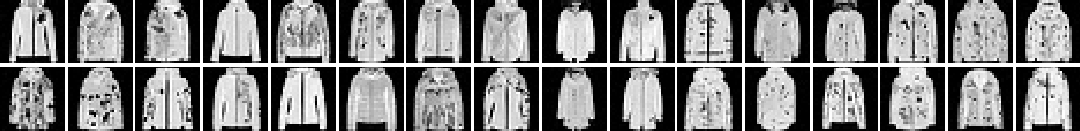} \\
 \raisebox{.3cm}{dress} & \includegraphics[trim={0 2.28cm 0 0},clip,width=0.88\textwidth]{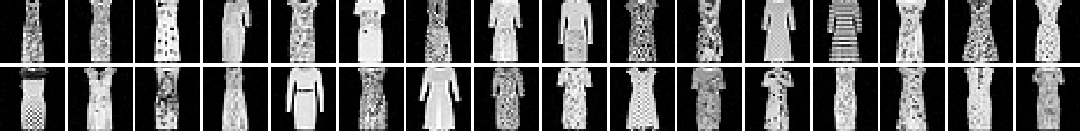} \\
 \raisebox{.3cm}{pullover} & \includegraphics[trim={0 2.28cm 0 0},clip,width=0.88\textwidth]{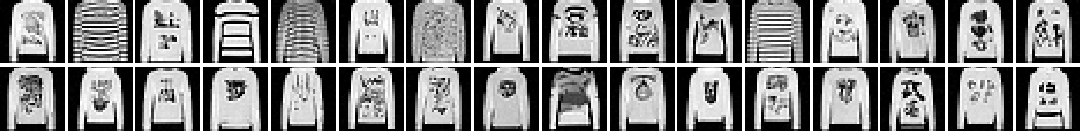} \\
 \raisebox{.3cm}{trouser} & \includegraphics[trim={0 2.28cm 0 0},clip,width=0.88\textwidth]{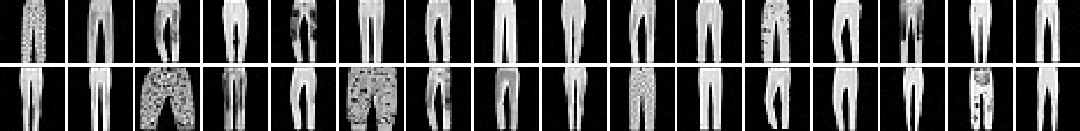} \\
 \raisebox{.3cm}{t-shirt} & \includegraphics[trim={0 2.28cm 0 0},clip,width=0.88\textwidth]{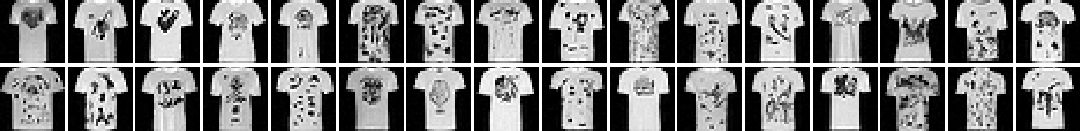}
\end{tabular}
\caption{Fashion MNIST synthetic samples generated by NCSN~\citep{song2019generative_ncsn} and pseudo-labels. Images are filtered based on a confidence threshold of $\tau = 0.95$ and categorized based on pseudo-labels. For each category, 16 random samples are shown.}
\label{fig:synth_examples_fmnist}
\end{figure*}

\vfill
% \clearpage\newpage
% \begin{figure*}[h!]
%  \centering
%   \includegraphics[trim={0 7cm 0 0},clip, width=0.71\textwidth]{images/samples_synth_cifar_4.pdf}
%  \caption{Synthetic samples per class from CIFAR-10 generative model. Images were categorized into classes based on their pseudo-labels, then for each class, we display 10 randomly sampled images from those which exceed the confidence threshold $\tau = 0.95$.}
%  \vspace{-5mm}
% \label{fig:synth_examples_cifar10}
% \end{figure*}

% \begin{figure*}[h!]
%  \centering
%   \includegraphics[trim={0 7cm 0 0},clip, width=0.71\textwidth]{images/samples_synth_fashion_1.pdf}
%  \caption{Synthetic samples per class from Fashion MNIST generative model. Images were categorized into classes based on their pseudo-labels, then for each class, we display 10 randomly sampled images from those which exceed the confidence threshold $\tau = 0.95$.}
%  \vspace{-5mm}
% \label{fig:synth_examples_fashion}
% \end{figure*}

%QNLI
\begin{table*}[h!]
\caption{\textbf{QNLI}: Two labeled examples, along with 3 nearest neighbors (based on RoBERTa representations) from our synthetic dataset. We include \textbf{labels} for original examples
    and \textbf{pseudo-labels} for synthetic examples in parenthesis.}
    \centering
    % % \small
    \scalebox{0.9}{
    \begin{tabular}{p{0.9\linewidth}}
    \toprule
        When did the third Digimon series begin? [SEP] Unlike the two seasons before it and most of the seasons that followed, Digimon Tamers takes a darker and more realistic approach to its story featuring Digimon who do not reincarnate after their deaths and more complex character development in the original Japanese. (\textbf{not entailment})\\
\midrule
KNN:\\
1: What is the name of the third season? [SEP] In addition to the first two seasons, the third season is the season that introduced new characters such as Captain Malice, a supervillain who became the antagonist in season two; and the villains known as the Heartbreakers, who introduced a group of crime fighters. (\textbf{not entailment})\\
2: When did the "Walking Dead" series end? [SEP] In 2013, AMC announced that it would develop a "superhero series", which would follow the storylines and characters from the "Walking Dead" series in order to bring the popular AMC original series to a new and younger audience. (\textbf{not entailment})\\
3: What is the main objective of the first season of the X-Files? [SEP] The first season was notable in that the characters were introduced and developed within the space of a single season, as was the format of the show itself. (\textbf{not entailment})\\
        \midrule\midrule
        What did Arsenal consider the yellow and blue colors to be after losing a FA Cup final wearing red and white? [SEP] Arsenal then competed in three consecutive FA Cup finals between 1978 and 1980 wearing their "lucky" yellow and blue strip, which remained the club's away strip until the release of a green and navy away kit in 1982–83.  (\textbf{entailment})\\
\midrule
KNN:\\
1: Who was the most important player for Arsenal Football Club in the 1950s? [SEP] Wenger continued to use Arsenal's famous red shirts and red kits throughout the 1950s and 1960s, and the red strip became the club's most recognised and recognizable symbol. (\textbf{not entailment})\\
2: When were the first two teams to play for the trophy in the Premier League? [SEP] The trophy was awarded to Manchester United in 1990-91 and was named after Sir Bobby Charlton, the club's manager until 1990, and later Sir Stanley Matthews, the club's most successful manager. (\textbf{not entailment})\\
3: What were the last four players to wear the yellow in the final? [SEP] With Arsenal having won all four major trophies in the period, they became the only club to have won five in a row. (\textbf{not entailment})\\
       \bottomrule
    \end{tabular}
    }
    \label{tab:qnli}
\end{table*}

%QQP
\begin{table*}[h!]
\caption{\textbf{QQP}: Two labeled examples, along with 3 nearest neighbors (based on RoBERTa representations) from our synthetic dataset. We include \textbf{labels} for original examples
    and \textbf{pseudo-labels} for synthetic examples in parenthesis.}
    \centering
    \small{
    \begin{tabular}{p{0.9\linewidth}}
    \toprule
       How is the life of a math student? Could you describe your own experiences? [SEP]   Which level of prepration is enough for the exam jlpt5? (\textbf{not duplicated})\\
       \midrule
       KNN: \\

1: What are the best courses for a mechanical engineering student? [SEP] What is the best course to do after completing a B.Tech in mechanical engineering? (\textbf{not duplicated})\\
2: How much marks are needed to get through the GATE with electronics? [SEP] What is the average score of the Gate EE exam? What are the cut-offs? (\textbf{not duplicated})\\
3: What is the best time table for students to prepare for IAS? [SEP] How can one study for IAS in a best time? (\textbf{not duplicated})\\
\midrule\midrule
How does an IQ test work and what is determined from an IQ test? [SEP] How does IQ test works? (\textbf{duplicated})\\
\midrule
KNN: \\
1: What is the average IQ of the U.S. population?  [SEP] How does an IQ test work? (\textbf{not duplicated})\\
2: Is the Iq test an effective way to measure intelligence? [SEP] How do IQ tests work? (\textbf{duplicated})\\
3: How is an IQ test on a scale from 1 to 100 scored? [SEP] How do you get your IQ tested? (\textbf{not duplicated})\\
       \bottomrule
         
    \end{tabular}
    }
    \label{tab:qqp}
\vspace{1cm}
\end{table*}

%RTE
\begin{table*}[h!]
 \caption{\textbf{RTE}: Two labeled examples, along with 3 nearest neighbors (based on RoBERTa representations) from our synthetic dataset. We include \textbf{labels} for original examples
    and \textbf{pseudo-labels} for synthetic examples in parenthesis.}
    \centering
    % \small{
    \scalebox{0.9}{
    \begin{tabular}{p{0.9\linewidth}}
    \toprule
        Like the United States, U.N. officials are also dismayed that Aristide killed a conference called by Prime Minister Robert Malval in Port-au-Prince in hopes of bringing all the feuding parties together. [SEP] Aristide had Prime Minister Robert Malval  murdered in Port-au-Prince. (\textbf{not entailment})\\
\midrule
KNN: \\
1: The government has been criticized for failing to prevent the mass protests that led to the ouster of President Nicolas Sarkozy earlier this month, which led to his second election defeat since assuming office two years ago. [SEP] Prime Minister Jean-Marc Ayrault is a former president of France. (\textbf{not entailment})\\
2: The French president, Jacques Chirac, has been urged by both the Vatican and the U.N. Security Council to step up efforts to prevent the return of former dictator Nicolas Sarkozy. [SEP] Nicolas Sarkozy left France. (\textbf{not entailment})\\
3: The French newspaper Le Monde says the French President Nicolas Sarkozy was advised by U.S. President George W. Bush about a possible trip to Iraq on Thursday. [SEP] Nicolas Sarkozy is a member of the United States. (\textbf{not entailment})\\
        \midrule\midrule
        Only a week after it had no comment on upping the storage capacity of its Hotmail e-mail service, Microsoft early Thursday announced it was boosting the allowance to 250MB to follow similar moves by rivals such as Google, Yahoo, and Lycos. [SEP] Microsoft's Hotmail has raised its storage capacity to 250MB. (\textbf{entailment})\\
\midrule
KNN: \\
1: The company, known as Microsoft Office, said it plans to sell all of the copies of its popular Office suite at a loss in the wake of the launch of Microsoft Windows 7, saying it will also make \$25 million in advertising costs, a move likely to hurt its long-standing position among consumers and business leaders. [SEP] Microsoft Office is a popular office suite. (\textbf{entailment})\\
2: The company's shares shot up more than 35\% after the company said it has sold all of its remaining inventory of the new Kindle e-readers at \$70 each. The shares rose to \$65.20 on Wednesday, their highest since March 6, 2011. ``The Kindle is our best selling product," said Jeff Bezos, founder and CEO of Amazon.com. [SEP] Amazon.com is based in Seattle. (\textbf{not entailment})\\
3: In response to concerns expressed by some investors, Microsoft last week said it would reduce the amount of shares that will be available to the public by 10 percent in the first quarter, with a further reduction to 3 percent in the second quarter. The stock price has plunged from \$24 to \$17, and Microsoft is currently offering \$17 to \$19 a share to its most senior employees. Some investors had criticized Microsoft's response to concerns about the price of its stock and about the perception that the company is in trouble. [SEP] Microsoft is struggling to sell its stock. (\textbf{not entailment})\\
       \bottomrule
         
    \end{tabular}
    }
    \label{tab:rte}
\vspace{2cm}
\end{table*}

%MRPC
\begin{table*}[h!]
\caption{\textbf{MRPC}: Two labeled examples, along with 3 nearest neighbors (based on RoBERTa representations) from our synthetic dataset. We include \textbf{labels} for original examples
    and \textbf{pseudo-labels} for synthetic examples in parenthesis.}
    \centering
    % \small
    \scalebox{0.9}{
    \begin{tabular}{p{0.9\linewidth}}
    \toprule
    A BMI of 25 or above is considered overweight ; 30 or above is considered obese . [SEP] A BMI between 18.5 and 24.9 is considered normal , over 25 is considered overweight and 30 or greater is defined as obese . (\textbf{paraphrase})\\
\midrule
KNN: \\
1: The report said that the average woman in her twenties who takes oral contraceptives daily can expect a loss of around 40 per cent of her bone density between the ages of 20 and 45 . [SEP] The study said the average woman in her twenties who used the pill every day , or every day for up to five years , can expect a loss of about 40 per cent of her bone density between the ages of 20 and 45 . (\textbf{paraphrase})\\
2: The report found that 17 percent of U.S. adults between ages 18 and 64 have a body mass index at or above the " normal " 20 . [SEP] For people of that age , 17.1 percent of adults have a body mass index at or above the " normal " 20 , while 12.6 percent have a body mass index of 30 or above . (\textbf{not paraphrase})\\
3: The survey shows the proportion of women between 20 and 44 who were obese was 6.3 percent , up from 5.7 percent in 2001 . [SEP] The proportion of women between 20 and 44 who were obese increased to 6.3 percent from 5.7 percent in 2001 . (\textbf{paraphrase})\\
        \midrule\midrule
        Shares of Genentech , a much larger company with several products on the market , rose more than 2 percent . [SEP] Shares of Xoma fell 16 percent in early trade , while shares of Genentech , a much larger company with several products on the market , were up 2 percent .(\textbf{not paraphrase})\\
\midrule
KNN: \\
1: Shares in Aventura fell as much as 5 percent , while shares in Medi-Cal climbed 2.5 percent . [SEP] Shares in Aventura were up 2.5 percent , while shares in Medi-Cal rose 2.5 percent . (\textbf{paraphrase})\\
2: Shares of Amgen rose \$ 2.29 , or 2.2 percent , to \$ 41.10 in after-hours trading . [SEP] Shares of Amgen , a division of Sanofi-Aventis , rose \$ 1.62 , or 1.6 percent , to \$ 41.06 in after-hours trading .(\textbf{paraphrase})\\
3: Shares of General Electric Co . GE.N rose more than 6 percent on the New York Stock Exchange , while shares of PepsiCo Inc . PEP.N rose 4.7 percent . [SPE] General Electric 's shares jumped almost 6 percent on the New York Stock Exchange , while PepsiCo 's climbed 4.7 percent . (\textbf{paraphrase})\\
       \bottomrule
         
    \end{tabular}
    }
    
    \label{tab:mrpc}
\end{table*}

%MNLI
\begin{table*}[h!]
\caption{\textbf{MNLI}: Two labeled examples, along with 3 nearest neighbors (based on RoBERTa representations) from our synthetic dataset. We include \textbf{labels} for original examples
    and \textbf{pseudo-labels} for synthetic examples in parenthesis.}
    \centering
    % \small{
    \scalebox{0.9}{
    \begin{tabular}{p{0.9\linewidth}}
    \toprule
    One of our number will carry out your instructions minutely. [SEP] A member of my team will execute your orders with immense precision. (\textbf{entailment})\\
\midrule
KNN: \\
1: We are at your disposal to help you with your investigation and provide a full range of pro bono services. [SEP] We are the only ones who can help you with your investigation. (\textbf{neutral})\\
2: I will speak with the chief officer of the contractor, who will be informed about the results of this effort. [SEP] The contractor is being informed about the results of the effort. (\textbf{entailment})\\
3: We have an office here to assist you. [SEP] An office is where we will assist you, said the manager. (\textbf{neutral})\\
  \midrule\midrule
  
Conceptually cream skimming has two basic dimensions - product and geography. [SEP] Product and geography are what make cream skimming work. (\textbf{neutral})\\
\midrule
KNN: \\
1: There are two main types of analysis and they are  the case study and the case report. [SEP] The case study is the most popular method used to analyze a subject. (\textbf{neutral})\\
2: A third approach to capturing and using this type of experience is to engage the program management and finance systems of the organization. [SEP] There are two strategies to capturing and using experience. (\textbf{contradiction})\\
3: The first is to see the basic elements of a business model in action. [SEP] Basic elements of business models are the most important for the success of any company. (\textbf{neutral})\\
       \midrule\midrule 
        I don't mean to be glib about your concerns, but if I were you, I might be more concerned about the near-term rate implications of this \$1. [SEP] I am concerned more about your issues than the near-term rate implications. (\textbf{contradiction}) \\
\midrule
KNN: \\
1: I'm not here to tell you of my own experiences, but they are important to others who might have similar concerns. [SEP] If you were to have similar concerns, I'd like to encourage you to tell them to me. (\textbf{neutral}) \\
2: I don't mean to sound judgmental, but as a person, I think that's an issue you're probably pretty much on your own if you think about it. [SEP] You're probably right if you think about it. (\textbf{neutral}) \\
3: But I don't mean to take your word for it. [SEP] I know you are correct, but I want to make sure it's clear that I do not agree. (\textbf{contradiction})\\
        
       \bottomrule
         
    \end{tabular}
    }
    \label{tab:mnli}
\end{table*}

%SST
\begin{table}[h!]
\caption{\textbf{SST-2}: Two labeled examples, along with 3 nearest neighbors (based on RoBERTa representations) from our synthetic dataset. We include \textbf{labels} for original examples
    and \textbf{pseudo-labels} for synthetic examples in parenthesis.}
    \centering
    % \small{
    \scalebox{0.9}{
    \begin{tabular}{p{0.9\linewidth}}
    \toprule
        are more deeply thought through than in most ` right-thinking ' films (\textbf{positive})\\
\midrule
KNN:\\
1: is far more sophisticated , insightful and thought-provoking than his previous films . (\textbf{positive})\\
2: is more sophisticated than its more obvious and less-than-dazzling counterparts (\textbf{positive})\\
3: is about as well-thought as the idea of a bad hair day , (\textbf{negative})\\
        \midrule\midrule
        contains no wit , only labored gags (\textbf{negative})\\
\midrule
KNN: \\
1: lacks insight , and lacks empathy (\textbf{negative})\\
2: has little humor or intelligence (\textbf{negative})\\
3: lacks all wit and humanity (\textbf{negative})\\
       \bottomrule
         
    \end{tabular}
    }

    \label{tab:sst2}
\end{table}

\clearpage

\section{Datasets}
\label{sec:datasets}

\input{tab-data}
\begin{table}[h!]
\caption{3 examples of input and labels for the Drybean tabular task.}
\small
    \centering
    %\small{
    \begin{tabular}{lcc}
    \toprule
             & \textbf{Attributes} & \textbf{Label} \\
    \midrule  %\midrule
     1 & 37316 , 718.059 , ... , 0.6738775377027459 , 0.9981482213213235 & SIRA\\
     2 & 50634 , 892.3919999999999 , ... , 0.48054883366111584 , 0.9942734696473365 & HOROZ\\
     3 & 33631 , 669.076 , ... ,  0.8466656241160356 , 0.9981796305487345& SEKER\\
%      en-de &4.2M & 3000 & 3003\\

     \bottomrule
    \end{tabular}
    %}
    %\vspace*{-.1cm}
    %\vspace*{-.1cm}
    \label{tab:connect4}
\end{table}

% \setlength\tabcolsep{1.5pt} % default value: 6pt
% \begin{wraptable}{r}{5.5cm}
% %\vspace{-2.5mm}
% %\begin{table}[h!]
% \small
%     \centering
%     \caption{\gal with soft \versus hard pseudo labels on GLUE dev sets.}
%     \begin{tabular}{lcccc}
%     \toprule
%             \textbf{Pseudo-label} & \textbf{SST-2} &  \textbf{RTE} & \textbf{MRPC} & \textbf{CoLA}\\
%             \midrule
%             hard &  95.0 &80.7 &90.8 &63.0 \\
%             soft &  95.3 & 81.4 & 91.7 & 65.1 \\
%     %\midrule % \midrule
% %      en-de &4.2M & 3000 & 3003\\
%     \bottomrule    
%     \end{tabular}
%     %\vspace{-.15cm}
%     \label{tab:self_logits}
%     \vspace{-4mm}
% %\end{table}
% \end{wraptable}

% \textbf{Soft v.s. hard pseudo label.} We investigate the use of soft and hard
% pseudo labels within the \gal framework for NLP.
% The results in \tabref{tab:self_logits} suggest that \gal using soft pseudo labels is more effective than hard labels on the GLUE benchmark.
% This finding is compatible with the intuition that soft labels enable
% measuring the functional similarity of neural networks better~\citep{hinton2015distilling}.

\section{Generating Synthetic Text for GLUE}
\label{sec:text:details}
To generate domain-specific synthetic data, we fine-tune GPT-2-large on the training set of each downstream task, excluding labels.
For tasks with multiple input sentences, we concatenate input sentences into a long sequences and separate sentences by special \textsc{[SEP]}
tokens. We generate new domain-specific data by using top-k random sampling similar to~\cite{radford2019language}.
We do not feed any prompt to the LM, but a special \textsc{[BOS]} token to initiate the generation chain.
A generation episode is terminated when a special \textsc{[EOS]} token is produced. 
We generate diverse sentences by varying the random seed.
After collecting enough synthetic data, we only retain unique sentences. 
For tasks with $\alpha$ input sentences,
we discard generated samples that violate this constraint (approximately 10\% of samples were rejected).

\textbf{Quality of synthetic dataset.}
%  (fidelity)
% while not memorizing to reproduce  exactly the sentences in the training corpus (novelty)
An effective generative model of text should learn the word preferences and genre associated with a given corpus, but still produce novel sentences.
In order to study the characteristics of our synthetic datasets, \tabref{tab:n_gram} reports the number of unique n-grams in the training and synthetic datasets, as well as the number of unique n-grams shared between them. %and shared n-grams for the training corpus as well as the synthetic data. 
%In addition, we also report the number of shared unique n-grams. 
%A large fraction of unigrams in the training datasets are included in the synthetic datasets
The high degree of overlap on uni-grams suggests that the fine-tuned GPT-2-large is somewhat domain-specific.
Meanwhile, the large number of unique n-grams in the synthetic dataset suggests that many novel word combinations are generated, which is helpful for \gal.

\begin{table}[h]
% \small 
\caption{For each dataset we report the number of unique n-grams in (the original dataset, the synthetic dataset, shared between the two).}
\centering
\scalebox{0.85}{

    \begin{tabular}{lccccc}
    \toprule
            & \textbf{SST-2} & \textbf{QNLI} & \textbf{RTE} &\textbf{MRPC} & \textbf{CoLA} \\
    \midrule  %\midrule
%      en-de &4.2M & 3000 & 3003\\
    1-gram	& (15k, 33k, 11k) &(89k, 231k, 55k) & (18k, 34k, 13k) & (15k, 27k, 10k) &(6k, 6k, 4k)\\
    %\midrule
    % 2-gram & 0.5477 & 0.4664 & 0.5031 & 0.4834 & 0.5096 & 0.4640 & 0.5095 & 0.3505 \\
    % \midrule
    3-gram &  (107k, 2M, 38k) &(2M, 10M, 513k)& (120k, 750k, 30k) & (105k, 562k, 27k) & (39k, 198k, 14k)\\
    % \midrule
    % 4-gram	& 0.1767 & 0.2732 & 0.1606 & 0.0947 & 0.2427 & 0.1219 & 0.2280 & 0.1122\\
    %\midrule
    5-gram & (109k, 4M, 9k) &(2M, 25M, 146k)& (130k, 1M, 4k)& 
    (120k, 1M, 7k) &
    (35k, 389k, 5k)\\
     \bottomrule
    \end{tabular}
    }
    % \caption{For each dataset we report number of unique n-grams for \textcolor{blue}{original} training dataset, \textcolor{red}{synthetic} dataset, and \textcolor{orange}{shared}. \red{\bf accessibility, appendix?}}
    %\vspace{-.1cm}
    %\vspace{-.3cm}
    \label{tab:n_gram}
\end{table}

\section{Importance of Pseudo-labels}
\label{app:pseudo_label}
We have argued and demonstrated that using class-conditional generative models to generate \textit{labeled} synthetic examples is less effective than \gal in \secref{sec:gal} and \secref{sec:expr}. To further verify this argument, we sample 100 instances from the synthetic RTE dataset generated by a class-conditional LM. Then we annotate these examples using a human annotator and the RoBERTa classifier. Finally, we compute the Accuracy, F1, Precision and Recall scores between human labels and RoBERTa labels, and between human labels and conditioning labels (i.e., labels that the class-conditional LM conditions on.). \tabref{tab:human_eval} shows that class-conditional LM has difficulty generating sentences retaining the semantics or pragmatics of a specified category, which also corroborates our theoretical analysis in \secref{sec:gal}. On the other hand, RoBERTa is able to produce higher quality labels that correlate better with human annotations.

\begin{table}[h!]
\small
\caption{Performance of RoBERTa annotation and conditioning labels on 100 random examples from the synthetic RTE dataset generated by a class-conditional LM.}
% \vspace{-.2cm}
    \centering
    \begin{tabular}{l@{\hspace{.25cm}}c@{\hspace{.25cm}}c@{\hspace{.25cm}}c@{\hspace{.25cm}}c}
    \toprule
             \textbf{Label type} & \textbf{Accuracy} &  \textbf{F1} & \textbf{Precision} & \textbf{Recall}\\
             \midrule
             RoBERTa  & 90.0  & 91.4  &  100.0 &  84.1 \\
     conditioning label & 72.0  & 71.4  &  66.0  & 77.8 \\ 

    %\midrule % \midrule
%      en-de &4.2M & 3000 & 3003\\
    \bottomrule    
    \end{tabular}
    % \vspace{-.3cm}
    %\vspace{-.1cm}
    \label{tab:human_eval}
\end{table}

\section{GPT-2 for classification}
\label{app:gpt2}
We have conducted additional experiments, where we fine-tune GPT-2 as a classifier. We have considered two variants of the GPT-2 model. The first varant is the original GPT-2 model (GPT2-original) pre-trained on open-domain text. The second variant is the GPT-2 model that was fine-tuned on the inputs of each task separately (GPT-2-finetuned). This model was used to generate task-specific (synthetic) unlabeled data. Finally, we also consider self-training with GAL on top of GPT2-original. Specifically, we use the GPT-2-finetuned model to synthesize 40x in-domain unlabeled data. Then we apply self-training to GPT-2-original, where the data is a combination of the original labeled data and pseudo-labeled synthetic data. \tabref{tab:gpt2-gal} suggests that the gains of \gal come from the pseudo-labeled synthetic data, \ie both synthetic unlabeled data and teacher's knowledge. Without the generation of synthetic unlabeled data, the domain-specific knowledge embedded in GPT-2-finetuned model cannot be utilized. As such, GPT-2-finetuned model is inferior to the GPT2-original model.

\input{tab-gpt2-gal}

\section{Training Details}
\label{sec:training_details}
We use the fairseq codebase~\citep{ott2019fairseq} for implementing both NLP and tabular experiments. Training details are summarized in \tabref{tab:training} and ~\tabref{tab:training_tab}. We use the HuggingFace codebase~\citep{wolf-etal-2020-transformers} for KD experiments. All NLP models are trained for 5 epochs with a learning rate of 2e-5 and a batch size of 32. All experiments are run on a single Nvidia V100 GPU.

\input{tab-training}

For the CV tasks, we first use the official implementation of NCSN ~\citep{song2019generative_ncsn} to generate the synthetic images for CIFAR-10 and Fashion MNIST. We use the pretrained checkpoints provided by the authors for the generation of synthetic CIFAR-10 images and we train a new generative model for Fashion MNIST from scratch with the same hyperparameters of the CIFAR-10 network. After generating the synthetic images, we apply \gal using a FixMatch-like setup~\citep{sohn2020fixmatch}, using the %We differ from FixMatch in that we do not include the labeled data (after removing their labels) into the unlabeled data pool. This is to avoid applying strong augmentations on the labeled data and thus ensure a fair comparison with the baseline. 
hyperparameters listed in \tabref{tab:training_cv}. We follow ~\citet{cubuk2020randaugment} for strong augmentations. Finally, the backbone of the classifiers is from this codebase: \url{https://github.com/bearpaw/pytorch-classification}. 

\input{tab-training-cv}
\section{Additional Details}
\label{sec:additional}
In Tables~\ref{tab:cv_stats_unfiltered}, and~\ref{tab:cv_stats_filtered}, we present some descriptive statistics of our CIFAR-10 synthetic image dataset to complement the samples shown in Figure~\ref{fig:synth_examples_cifar10} and to help shed some light on the nature of the images generated by the NCSN network. 
% Please add the following required packages to your document preamble:
% \usepackage{graphicx}
\begin{table}[h]
\caption{Unfiltered CIFAR-10 synthetic data statistics sorted by \emph{Count}. The \emph{Class} pseudo-label for each synthetic image is first obtained using a teacher model trained on the original CIFAR-10 data. \emph{Count} denotes the number of images per class in the entire synthetic dataset (500K images). \emph{Confidence} statistics shows the mean and standard deviation of the teacher model confidence score aggregated over each class.}
\centering
\begin{tabular}{cccc}
\toprule
\multicolumn{1}{l}{} & \multicolumn{1}{l}{} & \multicolumn{2}{l}{\textbf{Confidence}} \\
\textbf{Class}       & \textbf{Count}       & \textbf{Mean}       & \textbf{Std}      \\ \midrule
truck                & 64519                & 0.932               & 0.141             \\
ship                 & 32800                & 0.912               & 0.156             \\ 
horse                & 39604                & 0.916               & 0.158             \\
frog                 & 76194                & 0.887               & 0.168             \\
dog                  & 38784                & 0.826               & 0.188
\\
deer                 & 38829                & 0.865               & 0.183             \\
cat                  & 65969                & 0.826               & 0.185             
\\
bird                 & 37255                & 0.806               & 0.193             \\
car           & 36264                & 0.936               & 0.140             \\
airplane             & 69782                & 0.897               & 0.161             \\
\bottomrule
\end{tabular}%

\label{tab:cv_stats_unfiltered}
\end{table}
\newpage
% Please add the following required packages to your document preamble:
% \usepackage{graphicx}
\begin{table*}[h]
\caption{Filtered CIFAR-10 synthetic data statistics sorted by \emph{Count}. The \emph{Class} pseudo-label is first obtained for each synthetic image using a teacher model trained on the original CIFAR-10 data. The dataset is then filtered based on the teacher confidence score where only images with confidence $\geq \tau=0.95$ are retained. \emph{Count} denotes the number of images per class in the filtered synthetic dataset. \emph{Confidence} statistics shows the mean and standard deviation of the teacher model confidence score aggregated over each class.}
\centering
\begin{tabular}{cccc}
\toprule
\multicolumn{1}{l}{} & \multicolumn{1}{l}{} & \multicolumn{2}{l}{\textbf{Confidence}} \\
\textbf{Class}       & \textbf{Count}       & \textbf{Mean}       & \textbf{Std}      \\ \midrule
truck                & 48796                & 0.996               & 0.009             \\
ship                 & 22741                & 0.995               & 0.010             \\
horse                & 28498                & 0.996               & 0.010             \\
frog                 & 45923                & 0.993               & 0.012             \\
dog                  & 15984                & 0.989               & 0.014             \\
deer                 & 21413                & 0.993               & 0.012             \\
cat                  & 26311                & 0.988               & 0.014             \\
bird                 & 13440                & 0.988               & 0.014             \\
car           & 28329                & 0.997               & 0.008             \\
airplane             & 43745                & 0.992               & 0.012             \\
 \bottomrule
\end{tabular}%

\label{tab:cv_stats_filtered}
\end{table*}
